# Supplementary material for: Tightly Integrated Motion Classification and State Estimation in Foot-Mounted Navigation Systems
Source: arXiv:2305.09363 source file (2023-08-22)
Supplement: Supplementary file 1 [file appendix.tex]

\appendix
\section{Derivations}
\label{A:appendix1}
Derivation of expression for $p(y_n|y_{1:n-1})$ in \eqref{eq:pyyn}. By first writing $p(y_n|y_{1:n-1})$ as the marginal distribution of $p(y_n,x_n,\delta_n|y_{1:n-1})$ and then writing the result as a conditional distribution it holds that
\begin{equation}
  p(y_n|y_{1:n-1})\!=\!\sum_{\delta_n}\!\int_{x_n}\!\!\! p(y_n|x_n,\delta_n)p(x_n,\delta_n|y_{1:n-1})dx_n
\end{equation}
Next, writing $p(x_n,\delta_n|y_{1:n-1})$ as the marginal distribution of $p(x_n,\delta_n,x_{n-1},\delta_{n-1}|y_{1:n-1})$ and using the Markov properties of the signal model, it holds that
\begin{equation}
  \begin{split}
     &p(y_n|y_{1:n-1})\!=\!\sum_{\delta_n}\!\int_{x_n} \!\!\!p(y_n|x_n,\delta_n)\sum_{\delta_{n-1}}\!\int_{x_{n-1}}\!\!\!\!\!p(\delta_n|\delta_{n-1})\\
   &\cdot p(x_n|x_{n-1},\delta_{n-1}) p(x_{n-1},\delta_{n-1}|y_{1:n-1})dx_{n-1}dx_n
  \end{split}
\end{equation}
Next using that $p(x_{n-1},\delta_{n-1}|y_{1:n-1})=p(x_{n-1}|\delta_{n-1},y_{1:n-1})p(\delta_{n-1}|y_{1:n-1})$ and rewriting this in terms of the marginal distribution over $\delta_{1:n-2}$ yields
\begin{equation}\label{eq:py_y}
\begin{split}
  &p(y_n|y_{1:n-1})=\sum_{\delta_1,\ldots,\delta_n}p(\delta_n|\delta_{n-1})p(\delta_{1:n-1}|y_{1:n-1})\\
  &\cdot \int_{x_n}p(y_n|x_n,\delta_n)\int_{x_{n-1}}\!\!\!p(x_n|x_{n-1},\delta_{n-1})\\
  &\cdot p(x_{n-1}|\delta_{1:n-1},y_{1:n-1})dx_{n-1}dx_n
\end{split}
\end{equation}
Finally, if it holds that
\begin{equation}
\begin{split}
  &p(x_{n-1}|\delta_{1:n-1},y_{1:n-1})=\mathcal{N}\bigl(x_{n-1};\hat{x}_{n-1|n-1}^{\delta_{1:n-1}},P_{n-1|n-1}^{\delta_{1:n-1}}\bigr) \\
  & p(x_n|x_{n-1},\delta_{n-1})=\mathcal{N}\bigl(x_n;F_{n-1}x_{n-1},Q_n\bigr) \\
  & p(y_n|x_n,\delta_n)=\mathcal{N}\bigl(y_n;H_n x_{n},R(\delta_{n})\bigr),
\end{split}
\end{equation}
where $F_n$ and $H_n$ denote the Jacobian of $f(\cdot)$ and $h(\cdot)$, then %(see~\cite[p.93]{Bishop2006})
\begin{equation}\label{eq:N(y_y)}
\begin{split}
  & \int_{x_n}p(y_n|x_n,\delta_n)\int_{x_{n-1}}\!\!\!p(x_n|x_{n-1},\delta_{n-1})\\
  &\cdot p(x_{n-1}|\delta_{1:n-1},y_{1:n-1})dx_{n-1}dx_n\\
  &=\mathcal{N}\bigl(y_n;\hat{y}_{n|n-1}^{\delta_{1:n}},S_n^{\delta_{1:n}}\bigr)
\end{split}
\end{equation}
Here
\begin{equation}
  \hat{y}_{n|n-1}^{\delta_{1:n}}=H_n F_{n-1}\hat{x}_{n-1|n-1}^{\delta_{1:n-1}}
\end{equation}
\begin{equation}
   S_n^{\delta_{1:n}}=H_n P_{n|n-1}^{\delta_{1:n-1}}H_n^\top+R(\delta_{n})
\end{equation}
and
\begin{equation}
   P_{n|n-1}^{\delta_{1:n-1}}=F_{n-1}P_{n-1|n-1}^{\delta_{1:n-1}}F_{n-1}^\top+Q_n
\end{equation}
Combining \eqref{eq:py_y} and \eqref{eq:N(y_y)} yields the desired result.

%%% Local Variables:
%%% mode: latex
%%% TeX-master: "Main.tex"
%%% End:
